# Supplementary material for: Percival: Making In-Browser Perceptual Ad Blocking Practical With Deep Learning
Source: arXiv:1905.07444 source file (2020-05-20)
Supplement: Supplementary file 1 [file 9_appendix.tex]

\appendix
\section{Appendix}

\subsection{Additional Discussion}
\point{Deployment}
In this paper, we primarily focus on deploying \tool as a native in-browser ad-blocker. However, we note that this is not the only way to use our approach.  \tool can be used to build and enhance block lists for traditional ad blockers. For that we would need to set up a crawling infrastructure to find URLs and potentially DOM XPath expressions to block.

How to properly orchestrate crawling is not entirely clear: the simple approach of crawling a subset of the most popular sites such as those provided by Alexa will likely miss the long tail~---~unpopular sites that are not reached by such crawls but are reached by the long tail of users. However, we can still use such techniques to frequently update block lists automatically.

Yet a third approach is to collect URLs (and possibly XPath expressions) in the browser that are not already blocked by existing block lists, and then to crowd-source these from a variety of users.

However, all these techniques come with different user privacy trade-offs. Blocking too late in the pipeline (e.g. during rendering) provides context that opens the doors for machine learning based blocking techniques, sacrificing though the privacy of the user since the tracking mechanisms might have already run at this stage. On the other hand, blocking too early allows for higher privacy guarantees, but the blocking accuracy will depend on the effectiveness of the filter lists. We believe that a hybrid of rendering time and filter lists based blocking can help the creation of effective shields against ads that balance the trade-offs between accuracy and privacy.

\begin{figure}[tb]
    \centering
    \includegraphics[width=\columnwidth,height=0.7\columnwidth]{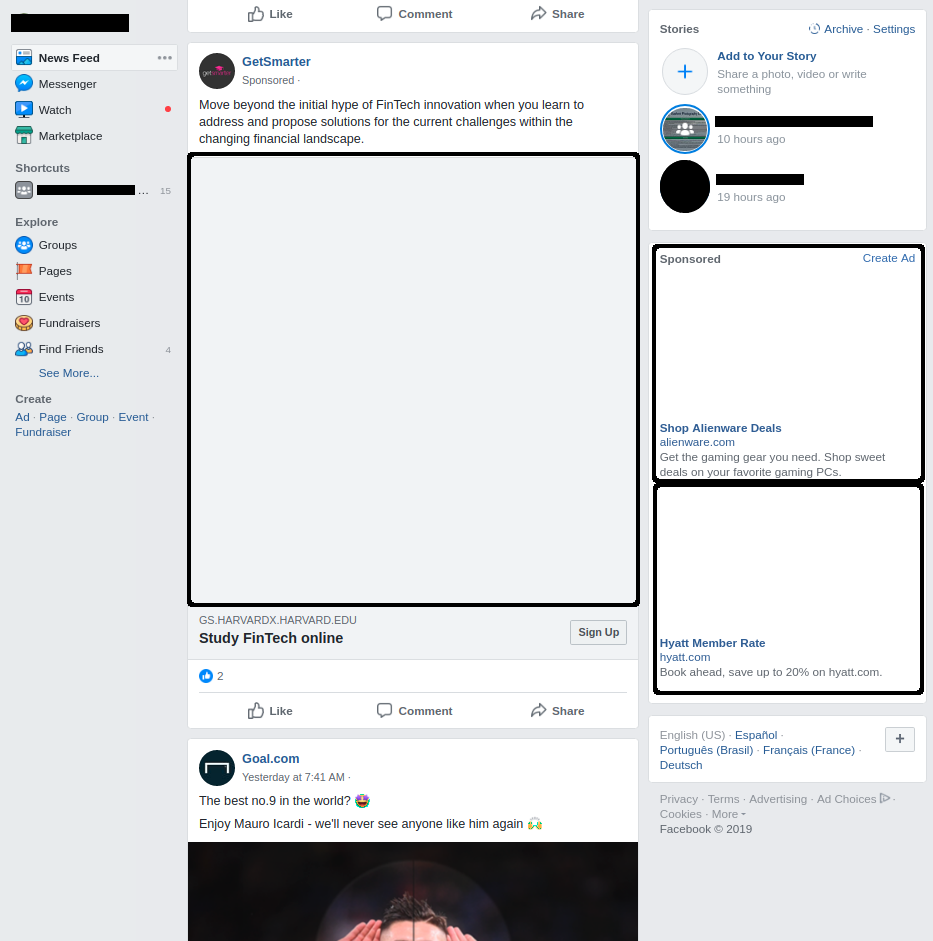}
    \caption{\tool blocking sponsored content embedded in the feed in addition to ads.}
    
\label{fig:deepbrave_facebook2}
\end{figure}

\begin{figure}[tb]
    \centering
    \includegraphics[width=\columnwidth,height=0.6\columnwidth]{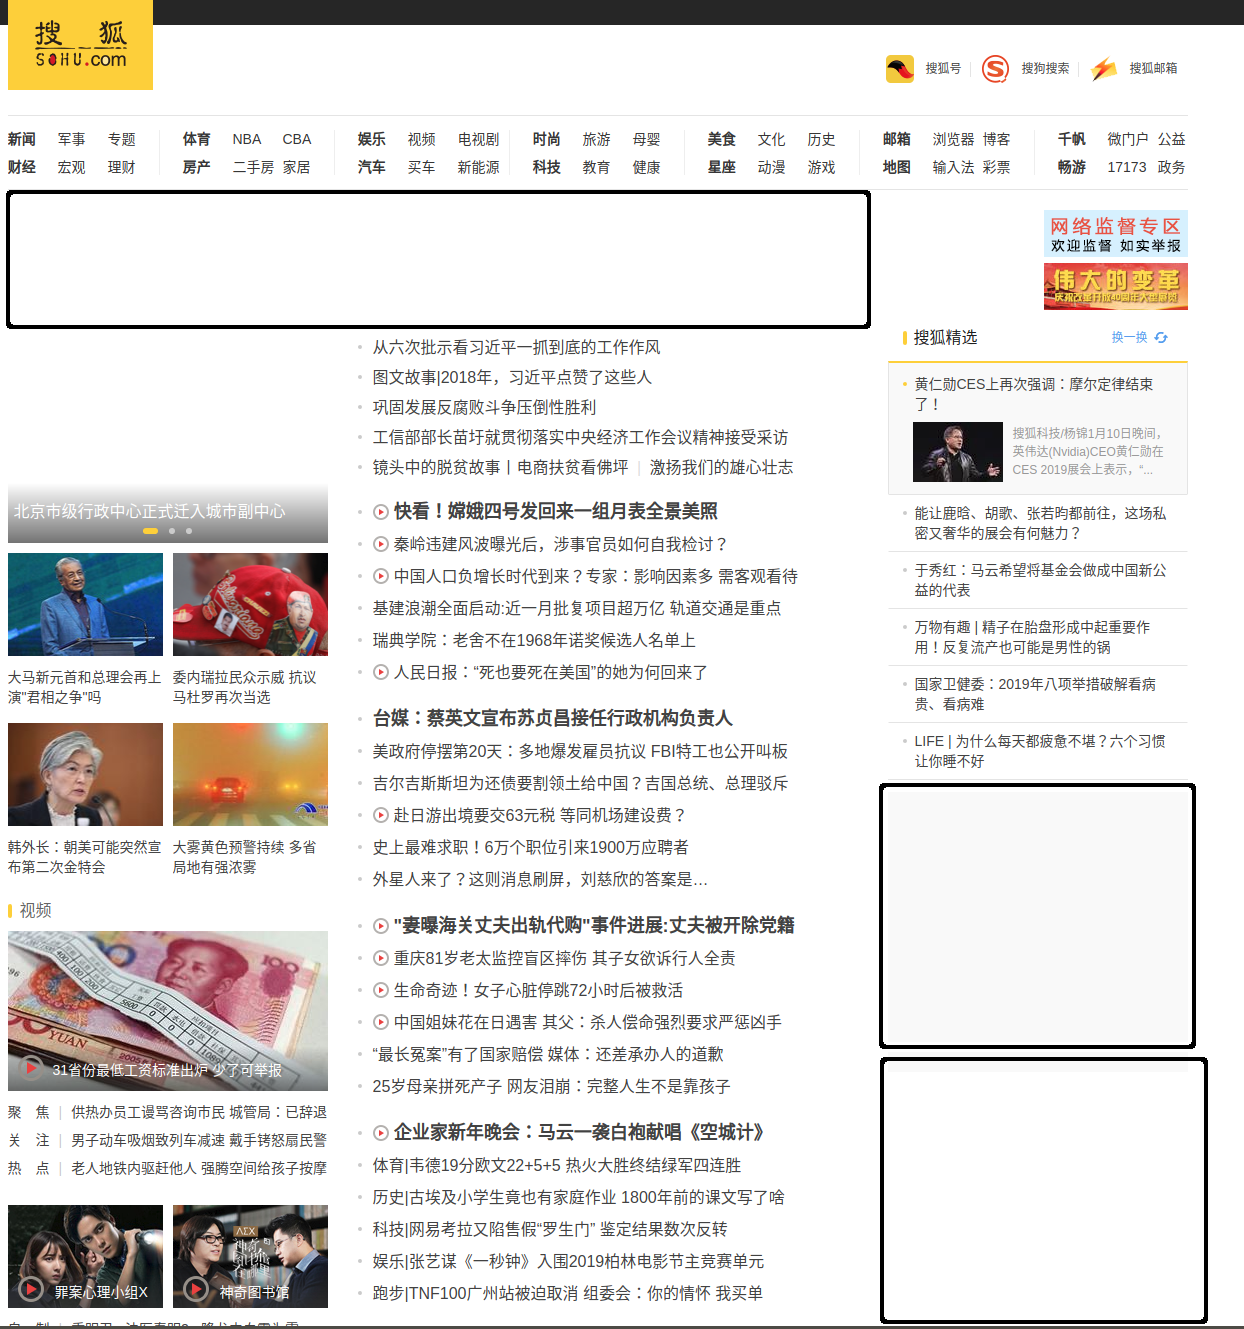}
    \caption{\tool results on \url{sohu.com} (Chinese language website).}
    \label{fig:deepbrave_china}
\end{figure}

\begin{figure}[tb]
\centering
    \includegraphics[width=\columnwidth]{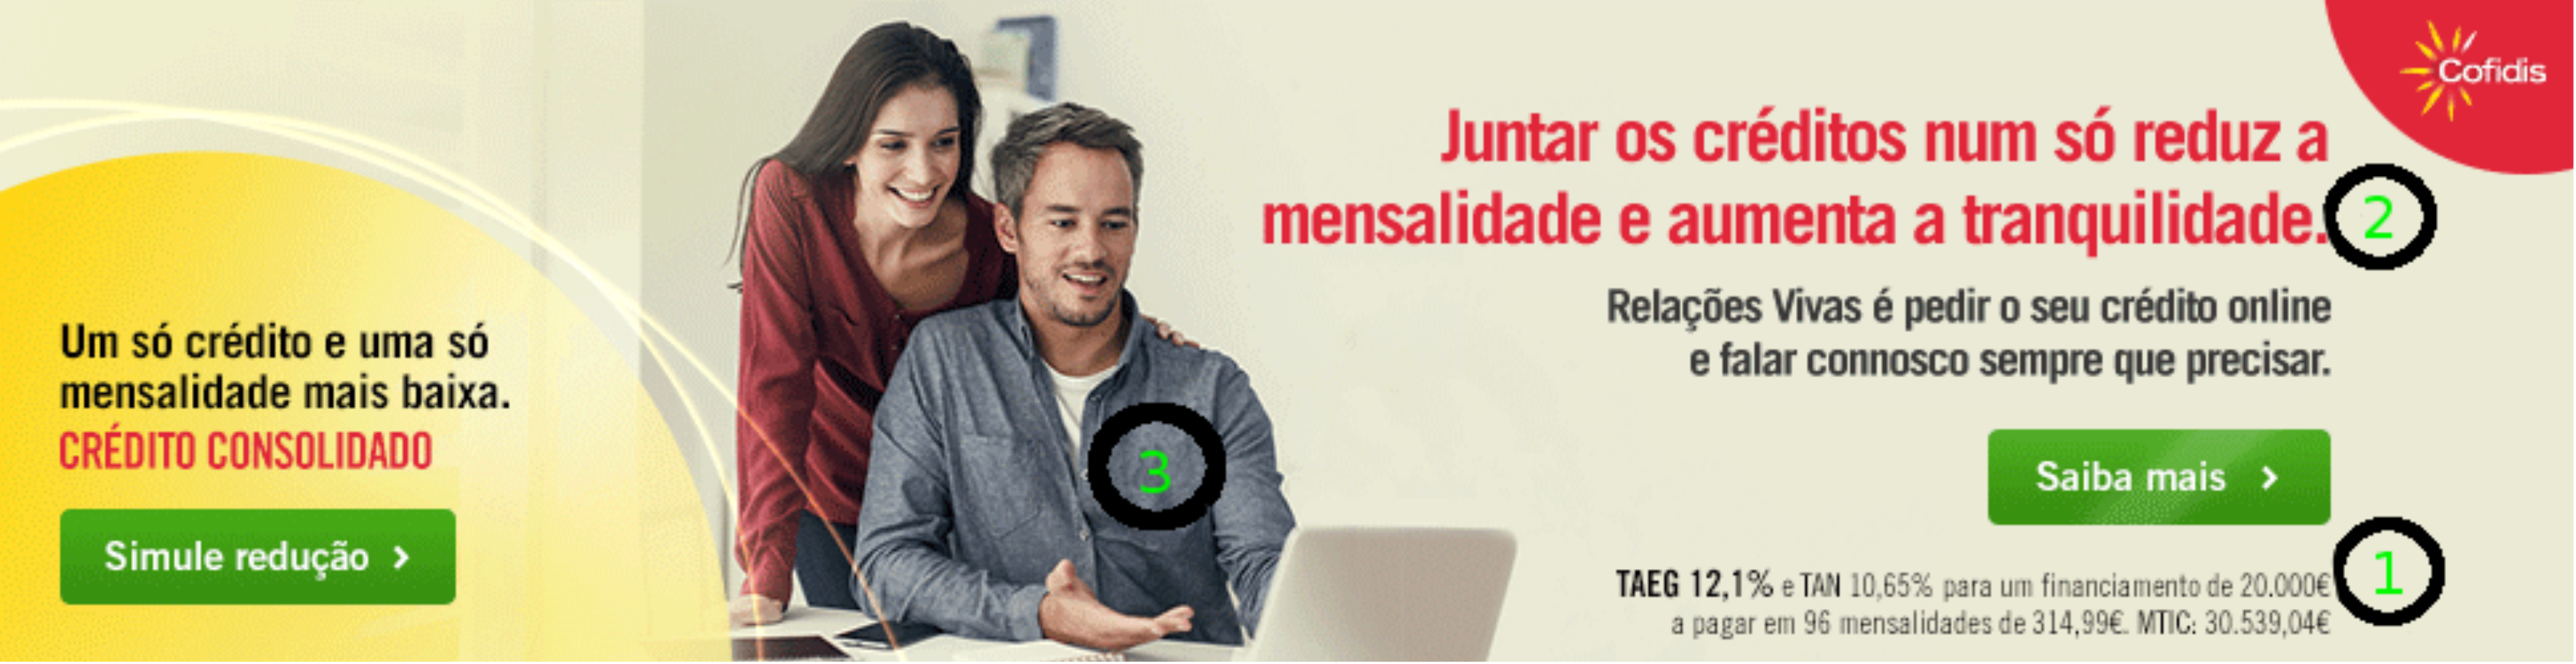}
    \caption{Example of an ad. Ads usually contain (1) body text, (2) image text, (3) ad image.}
    \label{fig:ad}
\end{figure}

\begin{figure}[tb]
    \centering
    \begin{subfigure}[t]{0.48\columnwidth}
        \centering
        \includegraphics[width=1\textwidth,height=0.7\textwidth]{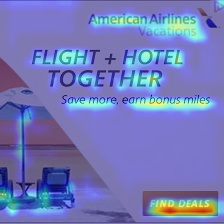}
        \caption{Ad image: Layer 5}
    \end{subfigure}
   ~ 
    \begin{subfigure}[t]{0.48\columnwidth}
        \centering
        \includegraphics[width=1\textwidth, height=0.7\textwidth]{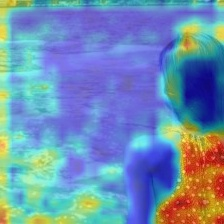}
        \caption{No Ad image: Layer 5}
    \end{subfigure}
    \caption{More examples of Salience map of the network on a sample ad and no-ad images. Each image corresponds to the output of Grad-CAM~\cite{SelvarajuDVCPB16} for the layer in question.}
    \label{ref:saliency2}
\end{figure}
